# Supplementary material for: Task-Aware Encoder Control for Deep Video Compression
Source: arXiv:2404.04848 source file (2024-04-20)
Supplement: Supplementary file 1 [file X_suppl.tex]

\clearpage
\setcounter{page}{1}
\maketitlesupplementary

\section{Implementation details of using DFS algorithm to find the optimal GoP structure for Bpp-mAP metric}

Different videos have different contents, and some of the contents are related to downstream machine vision tasks, including the size and quantity of objects, intensity of object movement, camera movement, etc. Considering these factors related to coding and downstream tasks, when trading off between the coding bitrate and downstream task performance, different videos must correspond to different optimal GoP structures. To explore the ``optimal GoP structures" and the upper bound of GoP structures using $P$ and $P_m$ frames, as shown in algorithm~\ref{alg:dfs}, we use a DFS algorithm to iterate over every possible structure for every GoP, which has a size of 10. In every GoP, we use the target function $R + \lambda L_{det}$ and find the GoP structure that leads to the minimum value of the target function. As shown in Fig.~\ref{fig:dfs}, the result of DFS shows a much better trade-off for the Bpp-mAP metric than the hand-craft ``DivGoP" structure. However, the time complexity of DFS is extremely high. For GoP size 10, there are 9 predicted frames, which means that the algorithm will visit $2^9=512$ nodes, and 512 times of encoding and decoding will be performed in each GoP. This obviously cannot be really applied. At the same time, the result of DFS does show that there is a huge gap between the hand-craft ``DivGoP" structure and optimal GoP structure. Therefore, how to use the inter-frame relationship, motion relationship and other information of the videos to dynamically determine the GoP structures more accurately within acceptable time complexity is a worth exploring question for us.

\begin{algorithm}
\caption{Using DFS to search for the optimal GoP structure on MOT}
\label{alg:dfs}
\begin{algorithmic}[1]
\Function{FindTargetPath}{$depth, path, min\_path, bpps, det\_losses, P_m$}
    \If{$depth > max\_depth$}
        \State \textbf{return}
    \EndIf
    \If{$P_m == True$}
    
        \State $bpp, det\_loss \gets codec.forward\_P_m$
        \State $path.append(0)$
        
        % \State Calculate bpp, mse, det\_loss
        \State $bpps.append(bpp)$
        \State $det\_losses.append(det\_loss)$
    \Else
        \State $bpp, det\_loss \gets codec.forward\_P$
        \State $path.append(0)$
        
        % \State Calculate bpp, mse, det\_loss
        \State $bpps.append(bpp)$
        \State $det\_losses.append(det\_loss)$
        \State \Comment{Update Reference frame}
    \EndIf
    \If{$depth == max\_depth$}
        % \State \Comment{Calculate the target function}
        \State $target \gets target\_function(bpps, det\_losses)$
        % \State \Comment{If the target function value is smaller, update the minimum path and minimum target value}
        \If{$target < min\_target$}
            \State $min\_path \gets current\_path$
            \State $min\_target \gets target$
        \EndIf
    \EndIf
    % \State \Comment{Recursively visit the left subtree and right subtree}
    \State \Call{FindTargetPath}{$depth + 1, ..., P_m=True$}
    \State \Call{FindTargetPath}{$depth + 1, ..., P_m=False$}
\EndFunction
\end{algorithmic}
\end{algorithm}

% \section{Ablation study of the GoP selection and mode prediction networks}

% We provide more ablation study results and visualization results in this section.
\begin{figure*}[t]
  \subfloat[]
  {\includegraphics[scale=0.31]{Figs/draw_mot_gop32_mota_supp.eps}}
  \subfloat[]
  {\includegraphics[scale=0.31]{Figs/draw_mot_gop32_motp_supp.eps}}
  \subfloat[]
  {\includegraphics[scale=0.31]{Figs/draw_mot_gop32_idf1_supp.eps}}
  \\
  \subfloat[]
  {\includegraphics[scale=0.31]{Figs/draw_mot_gop32_fn_supp.eps}}
  \subfloat[]
  {\includegraphics[scale=0.31]{Figs/rebuttal/draw_vod_deepsvc_rebuttal.eps}}
  \subfloat[]
  {\includegraphics[scale=0.31]{Figs/draw_psnr_gop12_classB_supp.eps}}
  \caption{(a) Bpp-MOTA curves on MOT Dataset. (b) Bpp-MOTP curves on HEVC ClassB dataset. (c) Bpp-IDF1 curves on MOT Dataset. (d) Bpp-FN curves on MOT Dataset. (e) Bpp-mAP curves on Imagenet VID dataset. (f) Bpp-PSNR curves on HEVC ClassB dataset.}
  \label{fig:supp_compare}
  \vspace{-0.1cm}
\end{figure*}

% \begin{figure*}[ht]
%   \centering
%   \subfloat
%   {\includegraphics[scale=0.31]{Figs/draw_vod_supp.eps}}
%   \subfloat
%   {\includegraphics[scale=0.31]{Figs/draw_psnr_gop12_classB_supp.eps}}
%   \caption{Left: Bpp-mAP curves on Imagenet VID dataset. Right: Bpp-PSNR curves on HEVC ClassB dataset.}
%   \label{fig:deepsvc}
% \end{figure*}

\section{Comparing with other one-to-one VCM methods}
In this section, we compare our method with existing one-to-one VCM methods in multi-object tracking and video object detection tasks.

For multi-object tracking task, we compare our method with SMC~\cite{tian2023non}, which is a ``one-to-one" VCM method. SMC contains two layers of encoders and decoders. The base layer is VVC and the semantic layer is designed to enhance the performance for downstream vision tasks. We requested the original authors of SMC to obtain the code and rigorously compared with it in our experimental settings. The results are shown in Fig.~\ref{fig:supp_compare}(a)(b)(c)(d). We compare our method with SMC in the metrics of MOTA, MOTP, IDF1 and FN. It is observed that out methods outperform SMC at bitrate range from around 0.04 to around 0.14. Our controlled TCM and controlled FVC still show the best and second-best performance.

We also compare our method with DeepSVC~\cite{lin2023deepsvc}. DeepSVC contains three layers of encoders and decoders, which are semantic layer,  structure layer and texture layer. The semantic layer serves downstream vision tasks, while structure and texture are used for the reconstruction task.

As for the video object detection task, we follow the experimental setting of DeepSVC, using the same detector TROIAlign~\cite{gong2021temporal} whose pre-trained weights are provided by mmtracking~\cite{mmtrack2020}. Specifically, we follow the data processing procedure of DeepSVC and compress the video frames using our method, then we feed the decoded frames to TROIAlign and evaluate the video object detection performance. The results are shown in Fig.~\ref{fig:supp_compare}(e). The ``Ours+TCM" method outperforms DeepSVC in this Bpp-mAP metric. Compared with DeepSVC, our method has two main strengths, on the one hand, our method is built on existing DVC codecs, making it both flexible and have the potential to use stronger DVC codecs to further demonstrate stronger performance. On the other hand, many video analysis methods use reference frame sampling strategy to enhance the video analysis performance. Some One-to-one VCM methods, such as DeepSVC, use feature decoder to support the video analysis task, making it difficult to still support the reference frame sampling strategy. Meanwhile, Our method is compatible with this strategy since we do not change the decoding procedure and still generate decoded video frames.

As for the video reconstruction task, we compare our methods with DeepSVC on HEVC Class B dataset. The result in Fig.~\ref{fig:supp_compare}(f) shows that our TCM still outperforms DeepSVC in Bpp-PSNR metric.

Our codec shows clear advantages over recent VCM methods such as SMC and DeepSVC: (1) Both SMC and DeepSVC require multiple decoders for different tasks, whereas our method necessitates only a single pre-trained decoder to support multiple tasks, which is more feasible to standardization and practical deployment. Once standardized and deployed in SoC, the decoder remains unchanged, allowing our codec to support new tasks without modifications. (2) As shown in Fig.~\ref{fig:supp_compare}, our method surpasses these competitors in MOT and VOD tasks in performance.

% Our method has two main strengths, on the one hand, our method is built on existing DVC codecs, making it both flexible and have the potential to use stronger DVC codecs to further demonstrate stronger performance. On the other hand, many video analysis methods use reference frame sampling strategy to enhance the video analysis performance. Some One-to-one VCM methods, such as DeepSVC, use feature decoder to support the video analysis task, making it difficult to still support the reference frame sampling strategy. Meanwhile, Our method is compatible with this strategy since we do not change the decoding procedure and still generate decoded video frames.

\section{Detail structure of autoregressive DVMP module}
\begin{figure}
  \centering
  \includegraphics[scale=0.5]{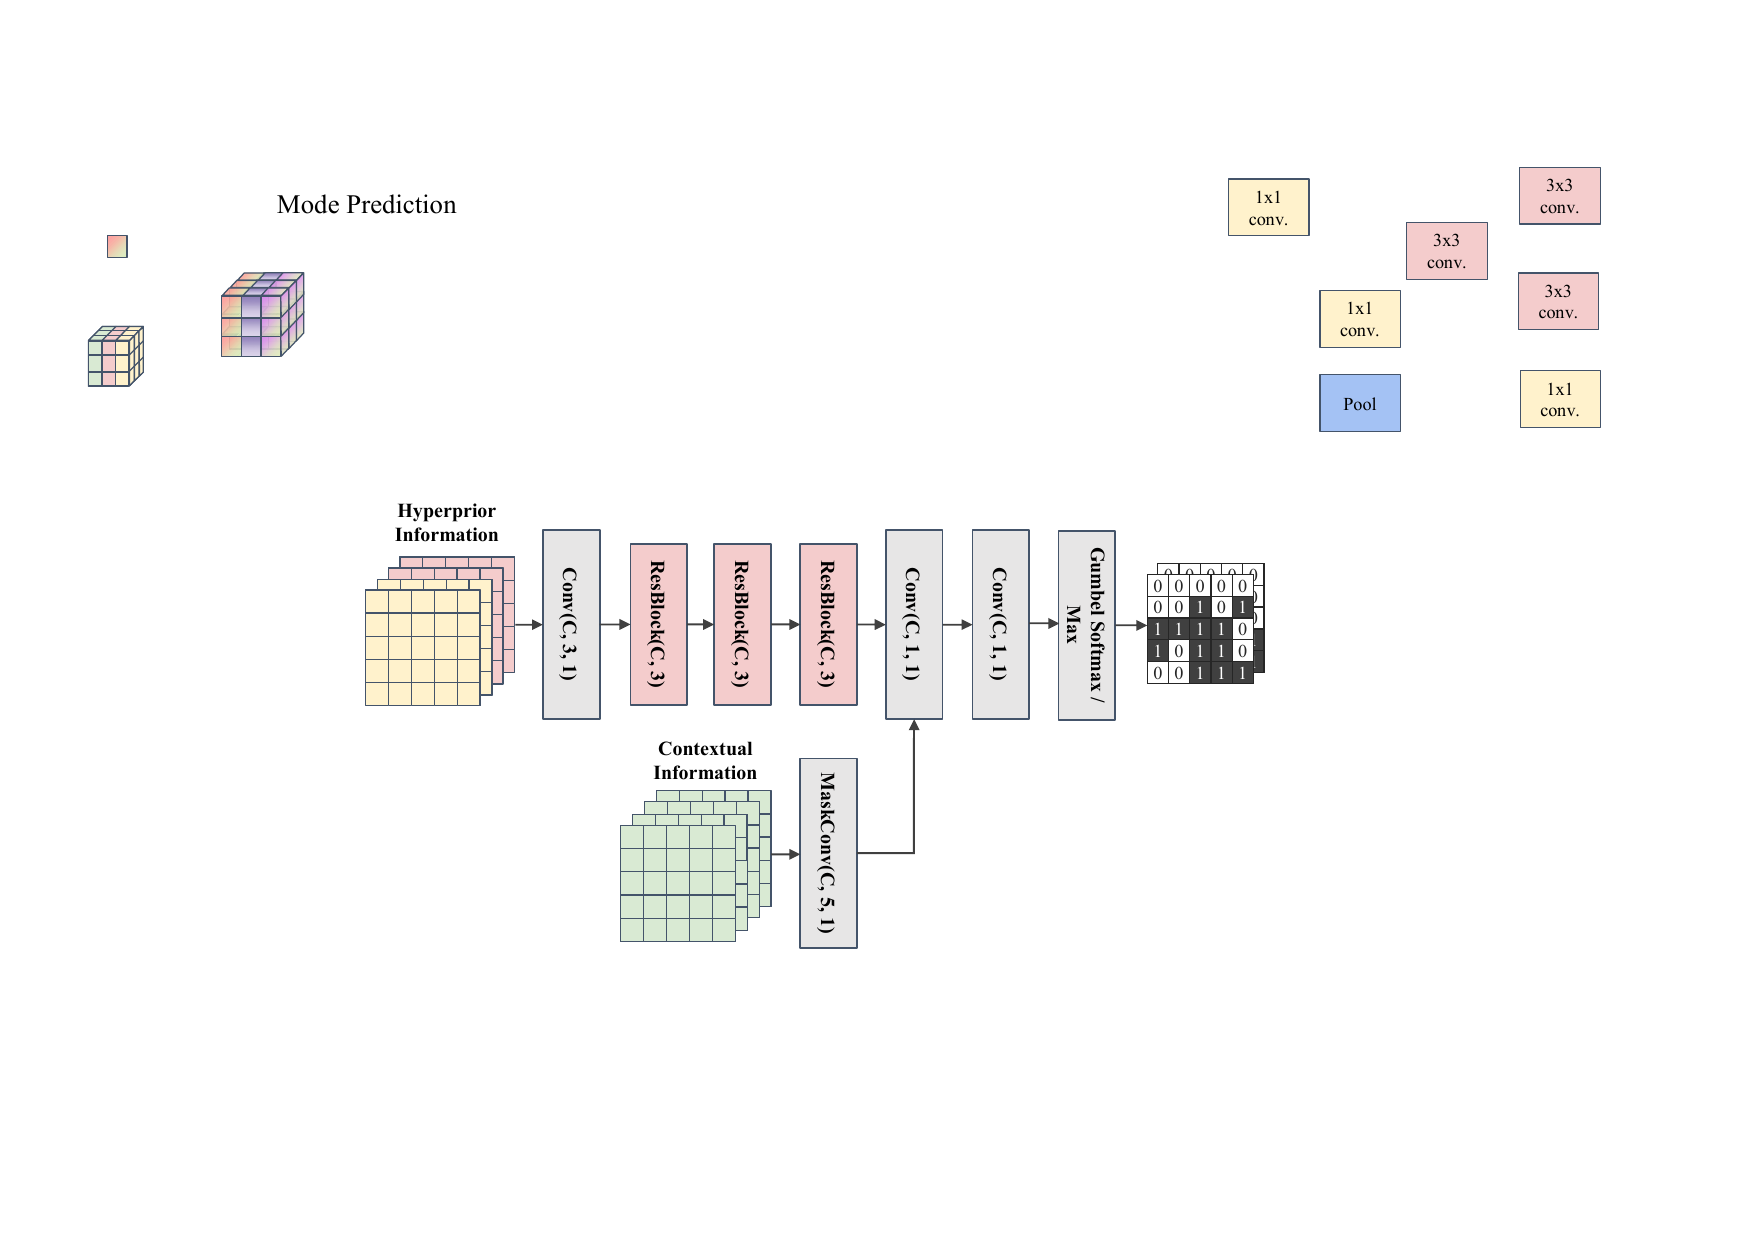}
  \caption{Autoregressive DVMP module.}
  \label{fig:supp_modeprediction}
  % \vspace{-0.5cm}
\end{figure}
As illustrated in Fig.~\ref{fig:supp_modeprediction}, we provide the structure of autoregressive DVMP module. The hyperprior network then predicts the mean and variance for each element, resulting in dimensions of $2c \times h \times w$. And the autoregressive networks predicts the contextual feature, which also has a shape of $2c \times h \times w$. The autoregressive DVMP firstly obtain the hyperprior information, undergoing one convolution layer and three ResBlocks with kernel size of $3$. Then the autoregressive convolution layer is used to handle the contextual information. After that, the two parts of feautures are concatenated and undergo two convolution layers with kernel size of $1$. In this way, our DVMP can achieve the support for mode prediction in DCVC. During training stage, we employ the Gumbel Softmax technique to predict the $m_t$. And during inference stage, we use max optain to generate the $m_t$.

\section{Discussion of extract and compress semantic information instead of whole video.} 
The idea of extracting and compressing semantic information to support downstream machine vision tasks is feasible, as evidenced by several existing methods~\cite{choi2022scalable,feng2022image}. 
% However, relying solely on compressed semantic information may be insufficient in complex scenes.
Nonetheless, in complex downstream scenarios, relying solely on compressed semantic information may be insufficient. Take autonomous driving as an example: multi-modal data, such as video, LIDAR, and radar, are imperative for precise decision-making. While semantic information like object detection is crucial, the video modality encompasses a broader context — including weather conditions and road quality — which can profoundly impact driving decisions. Furthermore, in practical applications, retaining video modality for purposes like secondary human inspection post-detection is often necessary. Therefore, our study maintains a focus on the video modality.

% We agree that extracting and compressing semantic information is feasible, as evidenced by several existing methods [4,10,22]. However, relying solely on compressed semantic information may be insufficient in complex downstream scenes, such as multi-modal applications. The video modality typically contains richer information; additionally, real-world applications often require video modality retention for purposes such as secondary human inspection of videos following detection. Therefore, this paper maintains a focus on the video modality.

% \section{Rationale}
% \label{sec:rationale}
% % 
% Having the supplementary compiled together with the main paper means that:
% % 
% \begin{itemize}
% \item The supplementary can back-reference sections of the main paper, for example, we can refer to \cref{sec:intro};
% \item The main paper can forward reference sub-sections within the supplementary explicitly (e.g. referring to a particular experiment); 
% \item When submitted to arXiv, the supplementary will already included at the end of the paper.
% \end{itemize}
% 
% To split the supplementary pages from the main paper, you can use \href{https://support.apple.com/en-ca/guide/preview/prvw11793/mac#:~:text=Delete%20a%20page%20from%20a,or%20choose%20Edit%20%3E%20Delete).}{Preview (on macOS)}, \href{https://www.adobe.com/acrobat/how-to/delete-pages-from-pdf.html#:~:text=Choose%20%E2%80%9CTools%E2%80%9D%20%3E%20%E2%80%9COrganize,or%20pages%20from%20the%20file.}{Adobe Acrobat} (on all OSs), as well as \href{https://superuser.com/questions/517986/is-it-possible-to-delete-some-pages-of-a-pdf-document}{command line tools}.
